# Supplementary material for: Remote capacitive sensing in two-dimension quantum-dot arrays
Source: arXiv:2005.14712 source file (2020-09-09)
Supplement: Supplementary file 1 [file floating_gate_paper_SM.pdf]

1 **Remote capacitive sensing in two dimension quantum dot array:**  
 2 **Supplementary Data**

3 Jingyu Duan,<sup>1,2,\*</sup> Michael A. Fogarty,<sup>1,2,†</sup> James Williams,<sup>1</sup>

4 Louis Hutin,<sup>3</sup> Maud Vinet,<sup>3</sup> and John J. L. Morton<sup>1,2,4</sup>

5 <sup>1</sup>*London Centre for Nanotechnology, University College London,*

6 *London WC1H 0AH, United Kingdom*

7 <sup>2</sup>*Quantum Motion Technologies, Nexus,*

8 *Discovery Way, Leeds, LS2 3AA, United Kingdom*

9 <sup>3</sup>*CEA, LETI, Minatec Campus, F-38054 Grenoble, France*

10 <sup>4</sup>*Dept. of Electronic & Electrical Engineering,*

11 *UCL, London WC1E 7JE, United Kingdom*

---

\* j.duan.17@ucl.ac.uk

† m.fogarty@ucl.ac.uk

## I. ADDITIONAL DEVICE DATA

The results from a number of devices are compiled to produce the data illustrated in Fig. 3 in the main text. Each device is configured with the same reflectometry measurement setup as illustrated in Fig. 1b). The core dimensions associated with the devices are depicted in Fig. S1a), where devices with floating gates are identical replications of the same  $2 \times 2$  bilinear array, with separation distance of  $D = 200\text{nm} - W$  as measured edge-to-edge from the nanowires, where  $W$  is the total nanowire width.

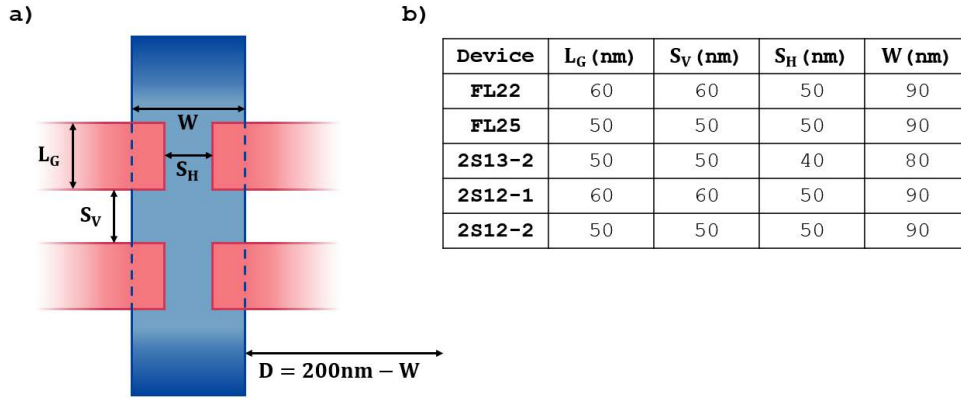

FIG. S1. a) Single nanowire with relevant dimensions indicated. b) Tabulated dimensions for different device used in this work

The core dimensions of the five different devices used to compile the data in the main text are tabulated in Fig. S1b). The two different devices which couple nanowires via floating gates are identified by the ‘FL’ key, while the remaining devices are simple  $2 \times 2$  bilinear arrays formed of a single nanowire.

An example of the operation of the  $2 \times 2$  array produces under an single nanowire is illustrated in the stability diagrams in Fig. S2, showing double-dot behavior for pairwise combinations of the four voltage control inputs, demonstrating controllability over the four dot locations. The stability diagrams are achieved by sweeping the relevant control inputs, while holding the remaining voltages low enough to de-populate the remaining dots of all electrons.

Fig. S2 from left to right shows loading first 6 electrons to  $D_{L2}, D_{R1}, D_{R2}$  in ‘2S13-2’ device, with dimensions listed in Fig. S1b). Capacitive shift of sensor dot  $D_{L1}$  probes other three quantum dots charge movement. A even stronger capacitive shift due to intentional ion-implanted donor appears in some of the stability diagram. The detailed study of donor-

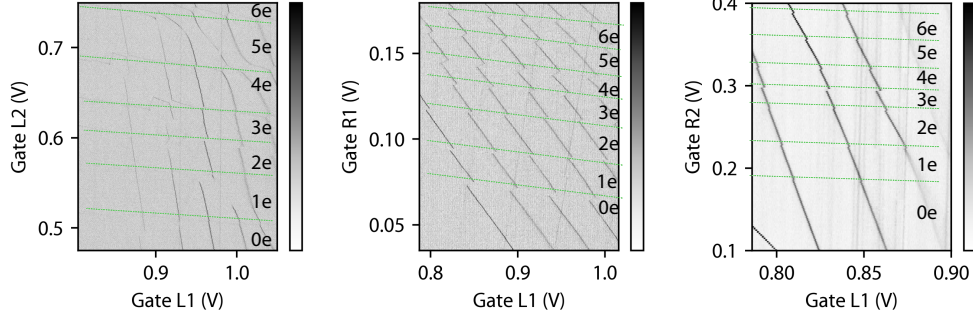

FIG. S2. Charge stability diagram of a 2S13-2 device, showing all three dot-sensor contributions individually operated in a double-dot regime

related interactions is out of the scope of this current work.

## II. SENSOR POWER BROADENING

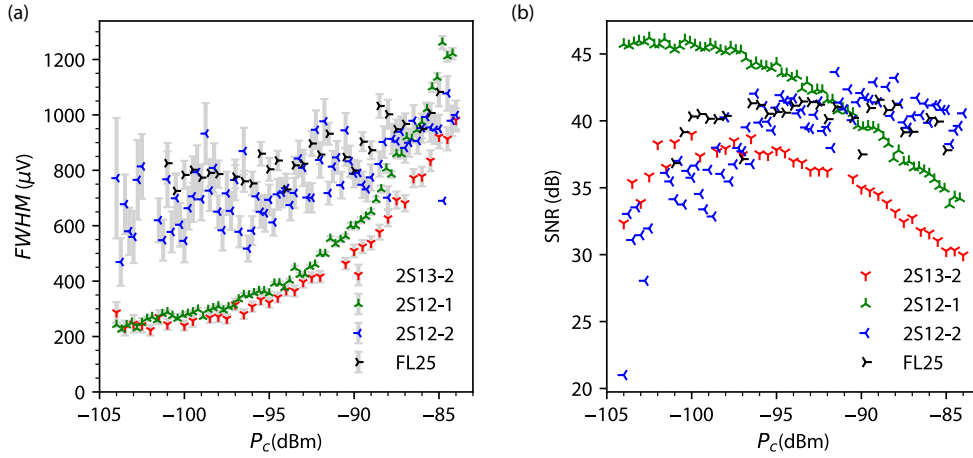

FIG. S3. (a) sensor dot-lead signal linewidth full width half maximum (FWHM) as a function of power delivered at device. (b) signal to noise ratio as a function of power delivered at device with integration time 0.4 ms.

We conduct power dependence experiments on different device sensor dot-lead coulomb peaks. We vary the input carriers power  $P_c$  at resonance frequency to observe the broadening of sensor linewidth  $FWHM$  and its impact on signal-to-noise ratio (SNR). SNR is defined as the  $SNR = S^2/\sigma_{bg}^2$  where  $S$  is the magnitude of the reflectometry coulomb peak and  $\sigma_{bg}$  is the standard deviation of the background noise. The recorded high SNR is a result of

41 long integration time.

42 As shown in Fig. ?? all four dot-lead linewidths are dominated by dot-lead tunnel rates  
 43 and near neighbour reservoir electron temperature when  $P_c < -90$  dBm. The selected dot-  
 44 lead transition of ‘FL25’ and ‘2S12-2’ experience much higher tunnel rates which in term  
 45 lead to lower SNR. When  $P_c > -90$  dBm, the dot-lead linewidths are dominated by the  
 46 input power to the reflectometry circuit, and SNR starts to degrade due to power induced  
 47 background noise.

### 48 III. CRYO-MOS SIMULATION DETAILS

49 The nanowire devices were modelled using the geometrical information given from the  
 50 fabrication dies. The electrostatics, semiconductor and Schrodinger-Poisson modules were  
 51 used within COMSOL to estimate the quantum dot size, electrostatics, capacitance matrices  
 52 and lever arms presented and contributing throughout this work.

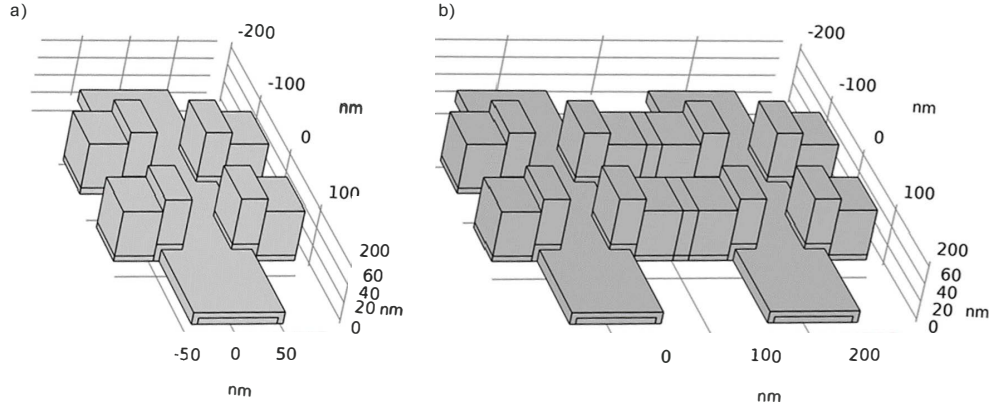

FIG. S4. a) Single nanowire 2x2 bilinear array and b) two parallel nanowires producing a 2x4 array of dots

53 Figure.S4 illustrates a single- and double-nanowire device of identical dimensions as con-  
 54 structed in COMSOL. The top gate metallic electrode  $G_T$  is not shown. The back-gate,  
 55 source and drain are held constant for all experiments, and are presumed to only add small  
 56 indirect coupling within the elements of the device and are not modelled accordingly.

57 To estimate the dot size, a Schrodinger and Poisson study is undertaken by transforming  
 58 the interface above the silicon into a boundary condition characterised by the material  
 59 properties including oxide thickness and material work functions. The gate inputs were

60 taken from experimental data, with the dot size resulting from the outputted probability  
61 density ( $\rho(x, y, z) = |\psi(x, y, z)|^2$ ), based on the calculate conduction band from the device  
62 simulated a T=2K, with the assumption that the electrons are fully confined inside the  
63 silicon nanowire. The quantum dot was then modelled as a perfect conductor ( $\epsilon_r = 1$ )  
64 within the device for use in the electrostatic simulation.

65 The collected dots and gates were then swept within an electrostatic study to find the  
66 full range of capacitance measurements needed to find the Maxwell capacitance matrix, in a  
67 model designed to replicate the full silicon chip. The lever arms for each terminal could the  
68 be measured using  $\alpha_{ij} = -C_{ij}/C_{ii}$ , with  $C_{ii}$  and  $C_{ij}$  being the self and mutual capacitance  
69 respectively.

70 Each parameter sweep investigated in the main text was generated as a symmetric device  
71 about the centre of the floating gate. For the case, of a variable Sv, Sh and nanowire to  
72 nanowire separation length; the dot size, gate overlap area and relative positions between  
73 these two features were fixed.

74 As the dots defined under the floating gates have stronger dependence on other voltage  
75 input parameters, such as  $V_T$  (see Supplementary § V for full discussion) it is possible that  
76 the dots under the floating gate have a different distribution of the electron wavefunction  
77 than that of a dot induced under a gate connected directly to an input control voltage.  
78 [More data to come?](#) To capture the effect of this within our simulations, the size of the  
79 dots underneath the floating gates are scaled until the relative ratio of the data in Fig. 2d)  
80 is achieved.

#### 81 **IV. 2×2 BILINEAR ARRAY CAPACITANCE AND LEVER ARM MATRIX**

82 From the simulations of the device shown in Fig. IIIa), the capacitance matrix is extracted  
83 and tabulated in Table S1.

84 Lever arm matrix which transforms voltage space from our vector of voltage control inputs  
85  $\mathbf{V}$ , to the vector of chemical potential on each dot  $\boldsymbol{\mu}$  takes the form  $\boldsymbol{\mu} = \boldsymbol{\alpha}\mathbf{V}$ , where elements  
86 of  $\boldsymbol{\alpha}$  are  $\alpha_{ij} = -C_{ij}/C_{ii}$ , and can be drawn from the values in Table S1:

TABLE S1. Maxwell capacitance matrix (aF) for the 2x2 bilinear array of quantum dots produced by a single nanowire.

|          | $G_{L1}$ | $G_{L2}$ | $G_{R1}$ | $G_{R2}$ | $D_{L1}$ | $D_{L2}$ | $D_{R1}$ | $D_{R2}$ | $GT$    |
|----------|----------|----------|----------|----------|----------|----------|----------|----------|---------|
| $G_{L1}$ | 41.1910  | -9.3116  | -8.7972  | -1.7283  | -5.4594  | -0.1128  | -0.3601  | -0.0669  | -6.1901 |
| $G_{L2}$ | -9.3120  | 41.1950  | -1.7229  | -8.8103  | -0.1131  | -5.4553  | -0.0672  | -0.3580  | -6.1917 |
| $G_{R1}$ | -8.7971  | -1.7230  | 41.2100  | -9.3153  | -0.3583  | -0.0669  | -5.4671  | -0.1125  | -6.1939 |
| $G_{R2}$ | -1.7281  | -8.8106  | -9.3152  | 41.2250  | -0.0671  | -0.3593  | -0.1133  | -5.4434  | -6.2043 |
| $D_{L1}$ | -5.4595  | -0.1130  | -0.3583  | -0.0671  | 6.4359   | -0.0073  | -0.0630  | -0.0056  | -0.0638 |
| $D_{L2}$ | -0.1128  | -5.4553  | -0.0669  | -0.3593  | -0.0073  | 6.4328   | -0.0056  | -0.0628  | -0.0640 |
| $D_{R1}$ | -0.3600  | -0.0672  | -5.4671  | -0.1133  | -0.0630  | -0.0056  | 6.4471   | -0.0073  | -0.0640 |
| $D_{R2}$ | -0.0669  | -0.3580  | -0.1126  | -5.4435  | -0.0056  | -0.0628  | -0.0073  | 6.4182   | -0.0638 |
| $GT$     | -6.1904  | -6.1917  | -6.1945  | -6.2038  | -0.0638  | -0.0639  | -0.0641  | -0.0638  | 95.4910 |

$$\begin{pmatrix} \mu_{L1} \\ \mu_{L2} \\ \mu_{R1} \\ \mu_{R2} \end{pmatrix} = 10^{-2} \begin{bmatrix} 13.2524 & 0.2743 & 0.8738 & 0.1624 \\ 0.2743 & 13.2524 & 0.1631 & 0.8689 \\ 0.8689 & 0.1624 & 13.2767 & 0.2743 \\ 0.1629 & 0.8714 & 0.2743 & 13.2039 \end{bmatrix} \begin{pmatrix} V_{L1} \\ V_{L2} \\ V_{R1} \\ V_{R2} \end{pmatrix} \quad (1)$$

Which seems to have a factor of 1.5 reduced in the diagonal elements when compared to the experimental data. From here, we can transform into a virtual gate space following the methods in Ref. [? ], where a change in the virtual voltage  $\Delta\tilde{\mathbf{V}}$  is mapped to change in the physical input voltages  $\Delta\mathbf{V}$  by means of the matrix  $\mathbf{B}$ , such that  $\Delta\mathbf{V} = \mathbf{B} \cdot \Delta\tilde{\mathbf{V}}$ . From the above capacitance matrix we find the following values for  $\mathbf{B}_{2 \times 2}^{sim}$ , compared to the experimentally derived values  $\mathbf{B}_{2 \times 2}^{exp}$

$$\mathbf{B}_{2 \times 2}^{sim} = \begin{bmatrix} 1.0048 & -0.0194 & -0.0657 & -0.0097 \\ -0.0194 & 1.0048 & -0.0097 & -0.0657 \\ -0.0654 & -0.0097 & 1.0048 & -0.0194 \\ -0.0097 & -0.0656 & -0.0193 & 1.0048 \end{bmatrix}, \quad \mathbf{B}_{2 \times 2}^{exp} = \begin{bmatrix} 1.241 & -0.0745 & -0.943 & 0.207 \\ -0.265 & 1.1165 & 0.212 & -0.630 \\ -0.302 & -0.1234 & 1.418 & -0.396 \\ 0.090 & -0.1340 & -0.605 & 1.273 \end{bmatrix} \quad (2)$$

where the effect of the aforementioned factor of 1.5 propagating to  $\mathbf{B}_{2 \times 2}^{sim}$  is between the

simulations and experiments is clearly visible. As proof of principle, we utilise the transformation matrix  $\mathbf{B}_{2 \times 2}^{exp}$  in order to produce the anti-crossing seen in Fig. S5.

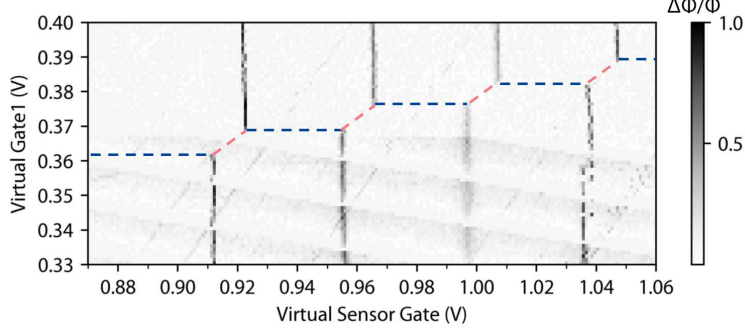

FIG. S5. Dot anticrossing produced in virtual gate space.

Here dashed lines are added as a guide to the eye for the second dot (blue) and inter-dot charge transitions (red), both which have tunnel rates outside the bandwidth of our reflectometry sensor. The remaining two dots are de-populated of any carriers. The diagonal background in this experiment is cross-talk from a parallel running setup on the same dilution refrigerator, with the abrupt disappearance of this periodic signal an indication of that experiment ending.

## V. $2 \times 4$ BILINEAR ARRAY CAPACITANCE AND LEVER ARM MATRIX

The study outlined in Supplemental Information IV can be expanded on to include the floating gate device illustrated in Fig. 1 of the main text, as shown in Fig. S4b). Here it is important to note that the overlying metallic gate electrode,  $G_T$ , can have a strong tuning effect upon the floating gates. As such, we expand the analysis to include it here, and the capacitance matrix between all elements of the  $2 \times 4$  array of quantum dots is illustrated in Table S2.

From this capacitance matrix, we can write the lever-arm matrix as a function of the metallic electrodes in Eq. V.

TABLE S2. Maxwell capacitance matrix (aF) for the 2x4 array of quantum dots comprised by two parallel running nanowires with interconnecting floating gates and overlying metallic top gate.

|           | $G_{L1}$ | $G_{L2}$ | $G_{F1}$ | $G_{F2}$ | $G_{R1}$ | $G_{R2}$ | $D_{L1}$ | $D_{L2}$ | $D_{FL1}$ | $D_{FL2}$ | $D_{FR1}$ | $D_{FR2}$ | $D_{R1}$ | $D_{R2}$ |
|-----------|----------|----------|----------|----------|----------|----------|----------|----------|-----------|-----------|-----------|-----------|----------|----------|
| $G_{L1}$  | 41.2290  | -9.3119  | -9.1290  | -1.7619  | -0.2990  | -0.1293  | -5.4703  | -0.1128  | -0.2142   | -0.0397   | -0.0091   | -0.0044   | -0.0101  | -0.0051  |
| $G_{L2}$  | -9.3119  | 41.2090  | -1.7555  | -9.1326  | -0.1293  | -0.2984  | -0.1130  | -5.4561  | -0.0394   | -0.2155   | -0.0044   | -0.0091   | -0.0051  | -0.0100  |
| $G_{F1}$  | -9.1287  | -1.7565  | 59.4500  | -14.6840 | -9.1218  | -1.7546  | -0.3854  | -0.0700  | -3.2852   | -0.0683   | -3.2999   | -0.0677   | -0.3858  | -0.0701  |
| $G_{F2}$  | -1.7631  | -9.1325  | -14.6840 | 59.5040  | -1.7647  | -9.1233  | -0.0700  | -0.3860  | -0.0678   | -3.3152   | -0.0679   | -3.2827   | -0.0701  | -0.3854  |
| $G_{R1}$  | -0.2990  | -0.1292  | -9.1225  | -1.7640  | 41.2300  | -9.3188  | -0.0101  | -0.0051  | -0.0091   | -0.0044   | -0.2138   | -0.0393   | -5.4641  | -0.1132  |
| $G_{R2}$  | -0.1292  | -0.2983  | -1.7538  | -9.1241  | -9.3188  | 41.2090  | -0.0051  | -0.0101  | -0.0044   | -0.0091   | -0.0394   | -0.2140   | -0.1129  | -5.4524  |
| $D_{L1}$  | -5.4703  | -0.1131  | -0.3855  | -0.0699  | -0.0100  | -0.0052  | 6.4449   | -0.0073  | -0.0384   | -0.0033   | -0.0006   | -0.0003   | -0.0006  | -0.0003  |
| $D_{L2}$  | -0.1129  | -5.4561  | -0.0699  | -0.3861  | -0.0052  | -0.0100  | -0.0073  | 6.4318   | -0.0033   | -0.0387   | -0.0003   | -0.0006   | -0.0003  | -0.0006  |
| $D_{FL1}$ | -0.2141  | -0.0394  | -3.2852  | -0.0678  | -0.0091  | -0.0044  | -0.0384  | -0.0033  | 3.8613    | -0.0025   | -0.0009   | -0.0004   | -0.0006  | -0.0003  |
| $D_{FL2}$ | -0.0396  | -0.2154  | -0.0683  | -3.3152  | -0.0045  | -0.0092  | -0.0033  | -0.0388  | -0.0025   | 3.8949    | -0.0004   | -0.0009   | -0.0004  | -0.0006  |
| $D_{FR1}$ | -0.0091  | -0.0044  | -3.3000  | -0.0679  | -0.2138  | -0.0393  | -0.0006  | -0.0003  | -0.0008   | -0.0004   | 3.8752    | -0.0025   | -0.0384  | -0.0033  |
| $D_{FR2}$ | -0.0044  | -0.0091  | -0.0676  | -3.2827  | -0.0393  | -0.2139  | -0.0003  | -0.0006  | -0.0004   | -0.0009   | -0.0025   | 3.8577    | -0.0033  | -0.0384  |
| $D_{R1}$  | -0.0100  | -0.0051  | -0.3859  | -0.0700  | -5.4641  | -0.1130  | -0.0006  | -0.0003  | -0.0006   | -0.0003   | -0.0384   | -0.0033   | 6.4393   | -0.0073  |
| $D_{R2}$  | -0.0051  | -0.0100  | -0.0700  | -0.3855  | -0.1132  | -5.4524  | -0.0003  | -0.0006  | -0.0003   | -0.0006   | -0.0033   | -0.0384   | -0.0073  | 6.4266   |
| $GT$      | -5.9392  | -5.9364  | -6.2505  | -6.2646  | -5.9416  | -5.9421  | -0.0549  | -0.0549  | -0.0286   | -0.0288   | -0.0285   | -0.0285   | -0.0549  | -0.0548  |

$$\begin{pmatrix} \mu_{L1} \\ \mu_{L2} \\ \mu_{FL1} \\ \mu_{FL2} \\ \mu_{FR1} \\ \mu_{FR2} \\ \mu_{R1} \\ \mu_{R2} \end{pmatrix} = 10^{-2} \begin{bmatrix} 13.2767 & 0.2743 & 0.6487 & 0.1175 & 0.0243 & 0.0125 & 0.0550 \\ 0.2743 & 13.2524 & 0.1175 & 0.6487 & 0.0125 & 0.0243 & 0.0550 \\ 0.5194 & 0.0956 & 5.5294 & 0.1139 & 0.0222 & 0.0108 & 0.0286 \\ 0.0961 & 0.5218 & 0.1148 & 5.5798 & 0.0108 & 0.0223 & 0.0287 \\ 0.0221 & 0.0107 & 5.5462 & 0.1141 & 0.5194 & 0.0954 & 0.0285 \\ 0.0107 & 0.0221 & 0.1136 & 5.5126 & 0.0954 & 0.5194 & 0.0285 \\ 0.0243 & 0.0125 & 0.6487 & 0.1176 & 13.2524 & 0.2743 & 0.0550 \\ 0.0125 & 0.0242 & 0.1176 & 0.6487 & 0.2743 & 13.2282 & 0.0548 \end{bmatrix} \begin{pmatrix} V_{L1} \\ V_{L2} \\ V_{F1} \\ V_{F2} \\ V_{R1} \\ V_{R2} \\ V_T \end{pmatrix} \quad (3)$$

111 which systematically falls under the same considerations discussed in Supplementary § IV.  
112 Under the assumption that the input voltages are pinned to their respective supplies, we  
113 can utilise the fact that the voltage on the floating gate electrodes is determined by the



capacitance matrix. As a first order approximation, we assume fully depleted dots, which results in the simplification of our virtual gate space to include only user controlled input voltages through the transformation:

$$\begin{pmatrix} V_{L1} \\ V_{L2} \\ V_{R1} \\ V_{R2} \\ V_{F1} \\ V_{F2} \\ V_T \end{pmatrix} = \begin{bmatrix} 1 & 0 & 0 & 0 & 0 \\ 0 & 1 & 0 & 0 & 0 \\ 0 & 0 & 1 & 0 & 0 \\ 0 & 0 & 0 & 1 & 0 \\ \alpha_{(G_{L1}, G_{F1})} & \alpha_{(G_{L2}, G_{F1})} & \alpha_{(G_{R1}, G_{F1})} & \alpha_{(G_{R2}, G_{F1})} & \alpha_{(G_T, G_{F1})} \\ \alpha_{(G_{L1}, G_{F2})} & \alpha_{(G_{L2}, G_{F2})} & \alpha_{(G_{R1}, G_{F2})} & \alpha_{(G_{R2}, G_{F2})} & \alpha_{(G_T, G_{F2})} \\ 0 & 0 & 0 & 0 & 1 \end{bmatrix} \begin{pmatrix} V_{L1} \\ V_{L2} \\ V_{R1} \\ V_{R2} \\ V_T \end{pmatrix} \quad (4)$$

where  $\alpha_{(i,j)} = C_{(i,j)}/C_{(j,j)}$  is the lever arm between electrodes. Hence, the transformation into a virtual gate space can be made here also, with the simulations yielding the control matrix  $B_{2 \times 4}^{sim}$ :

$$\begin{pmatrix} V_{L1} \\ V_{L2} \\ V_{R1} \\ V_{R2} \\ V_T \end{pmatrix} = \begin{bmatrix} 1.4736 & 0.5051 & 0.4715 & 0.5244 & -1.2183 & -1.3752 & -1.2305 & -1.3845 \\ 0.5006 & 1.4797 & 0.5195 & 0.4780 & -1.3628 & -1.2328 & -1.3429 & -1.2761 \\ 0.4727 & 0.5253 & 1.4723 & 0.5041 & -1.2556 & -1.3800 & -1.1931 & -1.3794 \\ 0.5188 & 0.4769 & 0.4973 & 1.4768 & -1.3626 & -1.2652 & -1.3330 & -1.2334 \\ -0.2813 & -0.2840 & -0.2807 & -0.2835 & 0.7187 & 0.7258 & 0.7058 & 0.7280 \end{bmatrix} \begin{pmatrix} \tilde{V}_{L1} \\ \tilde{V}_{L2} \\ \tilde{V}_{R1} \\ \tilde{V}_{R2} \\ \tilde{V}_{FL1} \\ \tilde{V}_{FL2} \\ \tilde{V}_{FR1} \\ \tilde{V}_{FR2} \end{pmatrix} \quad (5)$$

It can be seen from this virtual gate space matrix, that the  $G_T$  top gate plays a pivotal role in the tunability of the the floating gates, and dots defined beneath with respect to the surrounding electrodes.

123 **VI. CAPACITIVE EFFECTS OF THE FLOATING GATE: EXTENDED ANALY-**  
 124 **SIS**

125 In order to analyse the effect of the floating gate electrode, we take into account the second  
 126 order shift in the chemical potential of the sensor dot  $D_{L1}$  of the form sensor-FG-dot. We  
 127 treat the floating gate in a similar fashion to the dots from Ref. [21], while maintaining a  
 128 fixed charge to reflect the electrical isolation of the gate.

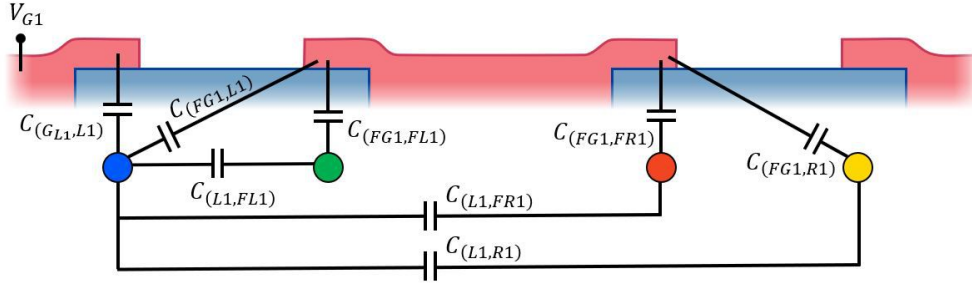

129 FIG. S6. Capacitive network illustrating the influence of the floating gate electrode  
 130

Following the analysis in Ref. [21], the first order sensor voltage shift due to the addition of an electron is given by:

$$\Delta V_{(L1, FL1)}^{(1)} = \frac{|e|}{C_{(G_{L1}, L1)}} \cdot \frac{C_{(L1, FL1)}}{C_{\Sigma FL1}} \quad (6)$$

$$\Delta V_{(L1, FR1)}^{(1)} = \frac{|e|}{C_{(G_{L1}, L1)}} \cdot \frac{C_{(L1, FR1)}}{C_{\Sigma FR1}} \quad (7)$$

$$\Delta V_{(L1, R1)}^{(1)} = \frac{|e|}{C_{(G_{L1}, L1)}} \cdot \frac{C_{(L1, R1)}}{C_{\Sigma R1}} \quad (8)$$

where the elements can be extracted from the Maxwell capacitance matrix, for each data-point in the parametric sweeps described in the main text. From Fig. S7, it can be seen that this first order effect is highly suppressed where there is a large separation between the dots, as the direct mutual capacitance between the dots and the SEB sensor  $D_{L1}$  rolls off within the indicated in the main text of  $\delta q \propto d^{-2.797}$  to  $d^{-1.816}$  (additional decay fits can be seen in Fig. S7). Most of these decays fall close to the  $d^{-3}$  dependence extracted for planar systems in silicon [23, 24]. It is noted that for these architectures there is a large amount of metallic electrodes present which can contribute to a screening effect of the charge. This is contrasted with the face-to-face decay rate of  $d^{-1.816}$ , where the majority of the metal between the two dots has been removed. If we now take the effective shift in the floating

gate into account we arrive at a second order approximation to the sensor voltage shift:

$$\Delta V_{(L1,FL1)}^{(2)} = \frac{|e|}{C_{(GL1,L1)}} \left[ \frac{C_{(L1,FL1)}}{C_{\Sigma FL1}} + \frac{C_{(L1,FG)}}{C_{\Sigma FG}} \cdot \frac{C_{(FG,FL1)}}{C_{\Sigma FL1}} \right] \quad (9)$$

$$\Delta V_{(L1,FR1)}^{(2)} = \frac{|e|}{C_{(GL1,L1)}} \left[ \frac{C_{(L1,FR1)}}{C_{\Sigma FR1}} + \frac{C_{(L1,FG)}}{C_{\Sigma FG}} \cdot \frac{C_{(FG,FR1)}}{C_{\Sigma FR1}} \right] \quad (10)$$

$$\Delta V_{(L1,R1)}^{(2)} = \frac{|e|}{C_{(GL1,L1)}} \left[ \frac{C_{(L1,R1)}}{C_{\Sigma R1}} + \frac{C_{(L1,FG)}}{C_{\Sigma FG}} \cdot \frac{C_{(FG,R1)}}{C_{\Sigma R1}} \right] \quad (11)$$

where the  $C_{(L1,FG)}$  term represents the coupling between the sensor and the floating gate, and  $C_{(FG,X)}/C_{\Sigma X}$  represents the charge capacitively induced on the floating gate, distributed by a factor of  $1/C_{\Sigma FG}$ . It is the total capacitance of the floating gate which is subject to geometrical dependencies upon the parameter sweeps. The comparisons within Fig. S7a) illustrates that, for sensing dots in the remote nanowire, the second-order contribution due to the floating gate is more dominant, giving rise to the advantage of the floating gate electrodes for long-range capacitive sensing.

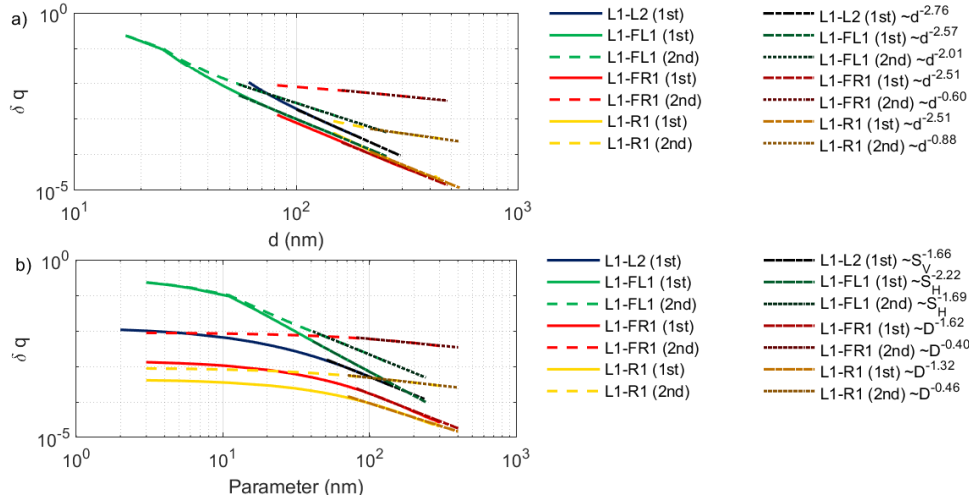

FIG. S7. a) Illustration of the first order and second order solutions to the detected charge on the sensor, normalised to sensor dot charge, as a function of the dot-dot separation. b) Illustrates the decay rate as a function of the design elements within the device architecture.

While the core aim of this manuscript is to compare the additional sensitivity to charge movements in remotely located quantum dots as facilitated by the floating gate, for completeness we include the second order enhancement to sensitivity to  $D_{FG1}$ . This element is not present for standard  $2 \times 2$  bilinear arrays formed of a single nanowire, where all electrodes are pinned to a supply voltage. Hence, the comparison made in the main text is between

143 the first order solution for  $d \propto$  extended  $W$  (i.e. sensing a face-to-face dot configuration  
 144 through silicon material) and the second order solution for the floating gate. The additional  
 145 sensitivity to dots in the  $D_{FG1}$  location can be seen as an additional enhancement advantage  
 146 which would not generally be present unless specifically interconnecting nanowires to form  
 147 larger arrays. While the dot-dot separation is well studied in the literature [23, 24], we  
 148 also wish to quantify the effects of the specific design parameters of the quantum device on  
 149 the mutual capacitance. As shown in Fig. S7b) we have re-scaled the x-axis so that it is  
 150 with respect to the input design parameters described in Fig. S4. Here we can see that the  
 151 trends plateau as each design parameter begins to approach the size of the quantum dot,  
 152 moving to a regime which would be physically challenging to realise in fabrication. The  
 153 reduction in sensitivity due to the input parameter follows a different trend when compared  
 154 to the dot-dot distance  $d$ . The reduction in sensitivity due to the face-to-face gap between  
 155 electrodes  $S_h$  is the largest, at  $dq \propto S_h^{-2.22}$ , reduced to  $dq \propto S_h^{-1.69}$  when the effect of the  
 156 floating gate directly above ont of the dots is taken into account. Comparatively, the  $S_v$   
 157 gap between the two gates along the nanowire gives rise to  $dq \propto S_v^{-1.66}$ . For the floating  
 158 gate, the dimensions of the floating gate contribute to the self-capacitance of the electrode  
 159 which, in turn, will contribute to the decay in sensitivity. For the floating gate geometry  
 160 in this work, we observe a  $dq \propto D^{-0.4}$ , however, this could be subject to further device  
 161 optimisation, outside the scope of this work, but touched on in Ref. [30].

- 
- 162 [1] J. Yoneda, K. Takeda, T. Otsuka, T. Nakajima, M. R. Delbecq, G. Allison, T. Honda,  
 163 T. Kodera, S. Oda, Y. Hoshi, N. Usami, K. M. Itoh, and S. Tarucha, Nat. Nanotechnol.  
 164 **13**, 102 (2018).  
 165 [2] X. Xue, T. F. Watson, J. Helsen, D. R. Ward, D. E. Savage, M. G. Lagally, S. N. Coppersmith,  
 166 M. A. Eriksson, S. Wehner, and L. M. K. Vandersypen, Phys. Rev. X **9**, 021011 (2019).  
 167 [3] D. M. Zajac, A. J. Sigillito, M. Russ, F. Borjans, J. M. Taylor, G. Burkard, and J. R. Petta,  
 168 Science (80-. ). **359**, 439 (2018).  
 169 [4] W. Huang, C. H. Yang, K. W. Chan, T. Tanttu, B. Hensen, R. C. C. Leon, M. A. Fogarty,  
 170 J. C. C. Hwang, F. E. Hudson, K. M. Itoh, A. Morello, A. Laucht, and A. S. Dzurak, Nature  
 171 **569**, 532 (2019).

- [5] M. A. Fogarty, K. W. Chan, B. Hensen, W. Huang, T. Tanttu, C. H. Yang, A. Laucht, M. Veldhorst, F. E. Hudson, K. M. Itoh, D. Culcer, T. D. Ladd, A. Morello, and A. S. Dzurak, *Nat. Commun.* **9** (2018), 10.1038/s41467-018-06039-x, arXiv:1708.03445.
- [6] L. M. K. Vandersypen, H. Bluhm, J. S. Clarke, A. S. Dzurak, R. Ishihara, A. Morello, D. J. Reilly, L. R. Schreiber, and M. Veldhorst, *npj Quantum Inf.* **3**, 34 (2017).
- [7] C. Jones, M. A. Fogarty, A. Morello, M. F. Gyure, A. S. Dzurak, and T. D. Ladd, *Physical Review X* **8**, 021058 (2018).
- [8] R. Maurand, X. Jehl, D. Kotekar-Patil, A. Corna, H. Bohuslavskyi, R. Laviéville, L. Hutin, S. Barraud, M. Vinet, M. Sanquer, and S. De Franceschi, *Nat. Commun.* **7** (2016), 10.1038/ncomms13575, arXiv:1605.07599.
- [9] M. Veldhorst, H. G. Eenink, C. H. Yang, and A. S. Dzurak, *Nat. Commun.* **8**, 1766 (2017), arXiv:1609.09700.
- [10] R. Li, L. Petit, D. P. Franke, J. P. Dehollain, J. Helsen, M. Steudtner, N. K. Thomas, Z. R. Yoscovits, K. J. Singh, S. Wehner, L. M. K. Vandersypen, J. S. Clarke, and M. Veldhorst, *Sci. Adv.* **4**, eaar3960 (2018).
- [11] Z. Cai, M. A. Fogarty, S. Schaal, S. Patomäki, S. C. Benjamin, and J. J. L. Morton, *Quantum* **3**, 212 (2019), arXiv:1904.10378.
- [12] B. Voisin, V.-H. Nguyen, J. Renard, X. Jehl, S. Barraud, F. Triozon, M. Vinet, I. Duchemin, Y.-M. Niquet, S. de Franceschi, and M. Sanquer, *Nano Lett.* **14**, 2094 (2014).
- [13] M. Urdampilleta, D. J. Niegemann, E. Chanrion, B. Jadot, C. Spence, P. A. Mortemousque, C. Bäuerle, L. Hutin, B. Bertrand, S. Barraud, R. Maurand, M. Sanquer, X. Jehl, S. De Franceschi, M. Vinet, and T. Meunier, *Nat. Nanotechnol.* **14**, 737 (2019).
- [14] M. G. House, I. Bartlett, P. Pakkiam, M. Koch, E. Peretz, J. Van Der Heijden, T. Kobayashi, S. Rogge, and M. Y. Simmons, *Phys. Rev. Appl.* **6**, 044016 (2016).
- [15] E. Chanrion, D. J. Niegemann, B. Bertrand, C. Spence, B. Jadot, J. Li, P.-A. Mortemousque, L. Hutin, R. Maurand, X. Jehl, M. Sanquer, S. De Franceschi, C. Bäuerle, F. Balestro, Y.-M. Niquet, M. Vinet, T. Meunier, and M. Urdampilleta, , 1 (2020), arXiv:2004.01009.
- [16] F. Ansaloni, A. Chatterjee, H. Bohuslavskyi, B. Bertrand, L. Hutin, M. Vinet, and F. Kuemmeth, (2020), arXiv:2004.00894.
- [17] V. N. Ciriano-Tejel, M. A. Fogarty, S. Schaal, L. Hutin, B. Bertrand, M. F. Gonzalez-Zalba, J. Li, Y. M. Niquet, M. Vinet, and J. J. L. Morton, , 1 (2020), arXiv:2005.07764.

- [18] I. H. Chan, R. M. Westervelt, K. D. Maranowski, and A. C. Gossard, *Appl. Phys. Lett.* **80**, 1818 (2002).
- [19] L. Hutin, R. Maurand, D. Kotekar-Patil, A. Corna, H. Bohuslavskyi, X. Jehl, S. Barraud, S. De Franceschi, M. Sanquer, and M. Vinet, in *2016 IEEE Symp. VLSI Technol.*, Vol. 2016-Septe (IEEE, 2016) pp. 1–2.
- [20] M. F. Gonzalez-Zalba, S. Barraud, A. J. Ferguson, and A. C. Betz, *Nat. Commun.* **6**, 6084 (2015).
- [21] W. G. van der Wiel, S. De Franceschi, J. M. Elzerman, T. Fujisawa, S. Tarucha, and L. P. Kouwenhoven, *Rev. Mod. Phys.* **75**, 1 (2002).
- [22] L. Trifunovic, O. Dial, M. Trif, J. R. Wootton, R. Abebe, A. Yacoby, and D. Loss, *Physical review X* **2**, 011006 (2012).
- [23] D. M. Zajac, T. M. Hazard, X. Mi, E. Nielsen, and J. R. Petta, *Phys. Rev. Appl.* **6**, 054013 (2016), 1607.07025.
- [24] S. F. Neyens, E. MacQuarrie, J. Dodson, J. Corrigan, N. Holman, B. Thorgrimsson, M. Palma, T. McJunkin, L. Edge, M. Friesen, S. Coppersmith, and M. Eriksson, *Phys. Rev. Appl.* **12**, 064049 (2019), arXiv:1907.08216.
- [25] M. D. Shulman, O. E. Dial, S. P. Harvey, H. Bluhm, V. Umansky, and A. Yacoby, *Science* (80-. ). **336**, 202 (2012).
- [26] H. O. Li, G. Cao, G. D. Yu, M. Xiao, G. C. Guo, H. W. Jiang, and G. P. Guo, *Nat. Commun.* **6**, 7681 (2015).
- [27] E. R. MacQuarrie, S. F. Neyens, J. P. Dodson, J. Corrigan, B. Thorgrimsson, N. Holman, M. Palma, L. F. Edge, M. Friesen, S. N. Coppersmith, and M. A. Eriksson, (2020), arXiv:2003.06768.
- [28] F. K. Malinowski, F. Martins, T. B. Smith, S. D. Bartlett, A. C. Doherty, P. D. Nissen, S. Fallahi, G. C. Gardner, M. J. Manfra, C. M. Marcus, and F. Kuemmeth, *Nat. Commun.* **10** (2019), 10.1038/s41467-019-09194-x.
- [29] F. Borjans, X. G. Croot, X. Mi, M. J. Gullans, and J. R. Petta, *Nature* **577**, 195 (2020).
- [30] L. Trifunovic, O. Dial, M. Trif, J. R. Wootton, R. Abebe, A. Yacoby, and D. Loss, *Phys. Rev. X* **2**, 011006 (2012).
- [31] N. Schuch and J. Siewert, *Phys. Rev. A* **67**, 032301 (2003).
- [32] T. Tantt, B. Hensen, K. W. Chan, C. H. Yang, W. W. Huang, M. Fogarty, F. Hudson,

234 K. Itoh, D. Culcer, A. Laucht, *et al.*, Physical Review X **9**, 021028 (2019).  
235 [33] W. Gilbert, A. Saraiva, W. H. Lim, C. H. Yang, A. Laucht, B. Bertrand, N. Rambal, L. Hutin,  
236 C. C. Escott, M. Vinet, and A. S. Dzurak, , 1 (2020), arXiv:2004.11558.
